# Supplementary material for: Topological Pathways to Two-Dimensional Quantum Turbulence
Source: arXiv:2411.11671 ancillary file (2025-09-04)
Supplement: Supplementary file 1 [file SuppMat.pdf]

# Supplemental material to: Topological Pathways to Two-Dimensional Quantum Turbulence

R. Panico,[1,2] G. Ciliberto,[3] G. I. Martone,[1,4] T. Congy,[5] D. Ballarini,[1] A. S. Lanotte,[1,4] and N. Pavloff[3,6]

[1] *CNR NANOTEC, Institute of Nanotechnology, Via Monteroni, 73100 Lecce, Italy*
[2] *Institut für Angewandte Physik, Universität Bonn, Wegelerstraße 8, 53115 Bonn, Germany*
[3] *Université Paris-Saclay, CNRS, LPTMS, 91405, Orsay, France*
[4] *INFN, Sezione di Lecce, 73100 Lecce, Italy*
[5] *Department of Mathematics, Physics and Electrical Engineering, Northumbria University, Newcastle upon Tyne NE1 8ST, United Kingdom*
[6] *Institut Universitaire de France (IUF)*

## METHODS

The experiment conducted utilized a planar $Al_xGa_{1-x}As$ microcavity containing 12 GaAs quantum wells, with aluminium fractions of 0.2 and 0.95 in the distributed Bragg reflectors, kept at a temperature of approximately 5 K. A ring potential, with a radius of ∼75 µm, is generated using an off-resonance CW laser beam ($\lambda = 735$ nm), shaped by a spatial light modulator displaying a Bessel function. This potential confines the polariton fluid by inducing a local energy blueshift in the polariton resonance due to the high exciton density under the CW pump. To inject the polariton fluid into the center of this potential, a pulsed laser (pulse duration of 2 ps) is focused into a Gaussian spot with a beam waist of approximately 17 µm. The excitation energy is slightly blue-detuned from the ground state by 1.2 meV (0.21 meV for the "low-energy" case reported in a later section), providing the polaritons with an initial kinetic energy that allows for their rapid expansion within the potential and subsequent hydrodynamic vortex formation upon collision with the potential barrier.

The time evolution of the polariton fluid is captured using off-axis digital holography, which involves the interference of the signal with a reference pulse (a sample of the excitation beam) with a variable time delay, enabling the retrieval of both the amplitude and phase of the fluid, as illustrated in Fig. S1. The temporal resolution is of around 1 ps and the spatial resolution is finer than the estimated healing length of the vortices. Each time frame is obtained by integrating over a large number of pulses, given the pulsed pump's repetition rate of 80 MHz and the typical integration time of 1 ms. Despite the averaging, spatial inhomogeneities allows for the observation of coherent vortex dynamics. To ensure statistical significance, the analysis averaged four measurements by translating the sample in-plane to eliminate morphological effects. Different spatial configurations can be observed at different sample locations, yet the statistical properties of the observables remain consistent. For each experimental condition and time frame, we identify vortices and critical points by computing the circulation around each point of the two-dimensional phase map and the corresponding velocity field, respectively, and searching for integer multiples of $2\pi$. From a simple comparison, we can further distinguish which of the critical points are nodes.

## BIFURCATION DETECTION

We give here a couple of examples of bifurcations such as those discussed in the main text, and detected during the time evolution of the experiment. The first is an instance where two nodes transform into a vortex-antivortex pair according to the mechanism in Eq. (2a) of the main text, which we recall here for completeness:

$$\text{node} + \text{node} \underset{b}{\overset{a}{\rightleftharpoons}} \text{vortex}_{(+)} + \text{vortex}_{(-)} \,. \qquad \text{(S1)}$$

In the left panel of Fig. S2, we present two consecutive time frames of the same spatial region, highlighting the evolution of the flow pattern from a configuration containing nodes and saddles (at $t = 15$ ps) to one where two nodes are transformed into a vortex and an antivortex ($t = 16$ ps).

In the right panel of Fig. S2, the Bristol annihilation mechanism [Eq. (5) of the main text, reproduced here]

$$\text{vortex}_{(+)} + \text{vortex}_{(-)} + \text{saddle} + \text{saddle} \underset{f}{\overset{e}{\rightleftharpoons}} \varnothing \,, \qquad \text{(S2)}$$

is observed in our experiment during the second stage of the dynamics, when dissipation begins to dominate ($t > t_c = 56$ ps). Two consecutive frames (at times $t = 76$ and $t = 77$ ps) illustrate the simultaneous annihilation of two saddles and a vortex-antivortex pair within a laminar plane flow, marking the dissipation of incompressible kinetic energy from the system.

## VORTEX CLUSTERING

In the main text, we discussed the crossover time $t_c$ at which the number or vortices, initially increasing significantly in the turbulent regime, starts a rapid decay. This time is non universal and depends on the initial configuration of the system. However, the survey of different

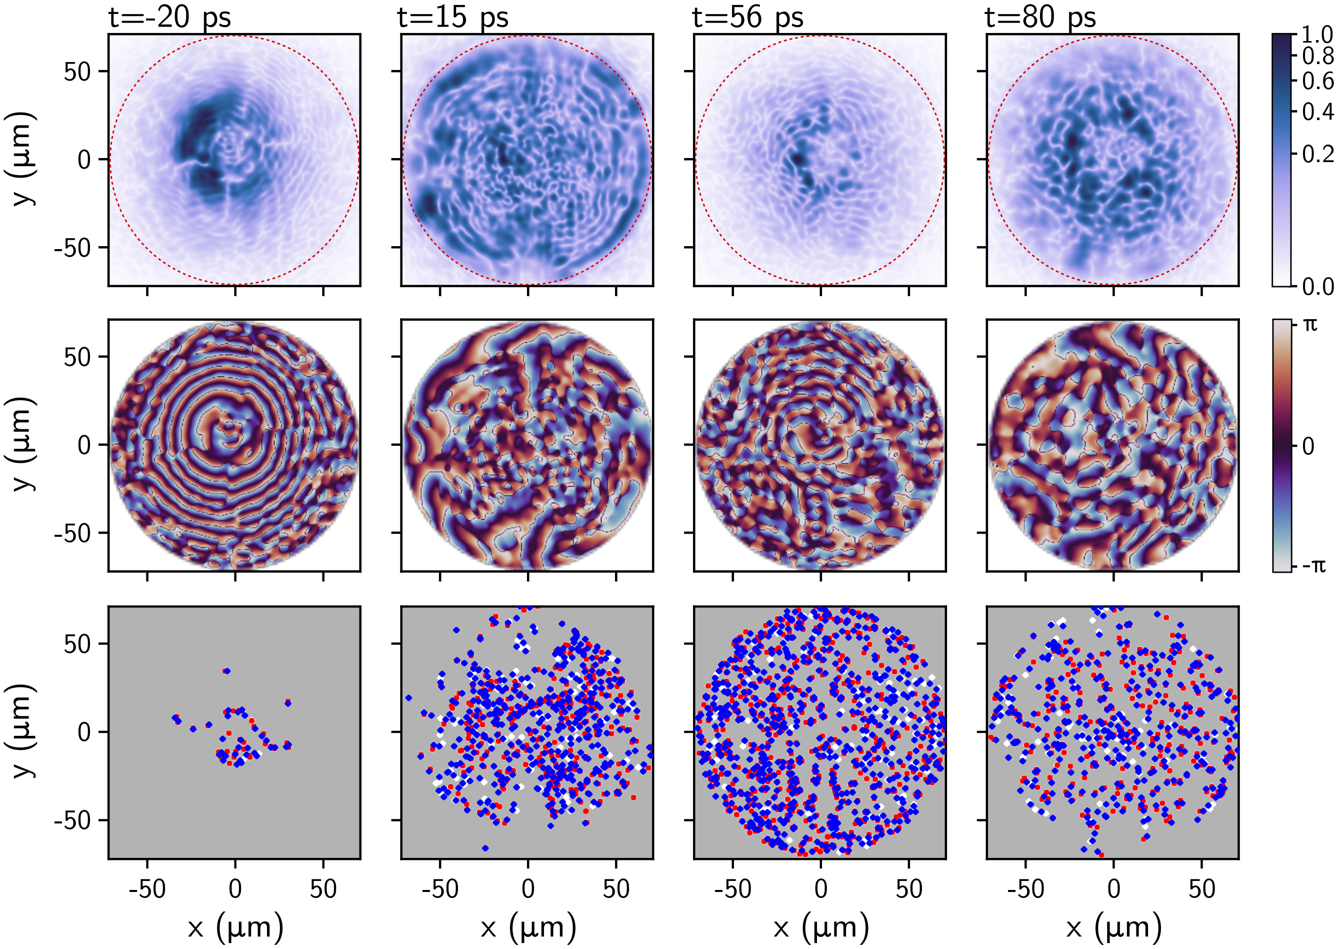


FIG. S1. Measured density (top), phase (middle), and critical points (bottom) of the polariton fluid for the high-energy case. At each time frame, the density is normalized to ensure its maximum value is 1. The dashed red circle represents the position of the confining potential. In the bottom row the white diamonds are nodes, the blue ones are saddles, and the red points are vortices (their signs are omitted for legibility). The time frames, from left to right, correspond to: the initial experimental condition ($t = -20$ ps), when the polariton fluid is still mostly localized in the center of the potential and has yet to fill all the available space; $t = 15$ ps after the sudden growth in the number of vortices, when the polariton fluid is flowing back after hitting the boundaries; the switching point at around $t = 56$ ps, when vortex growth stops and the Bristol mechanism becomes relevant; and finally, a snapshot near the end of the dynamics at $t = 80$ ps.

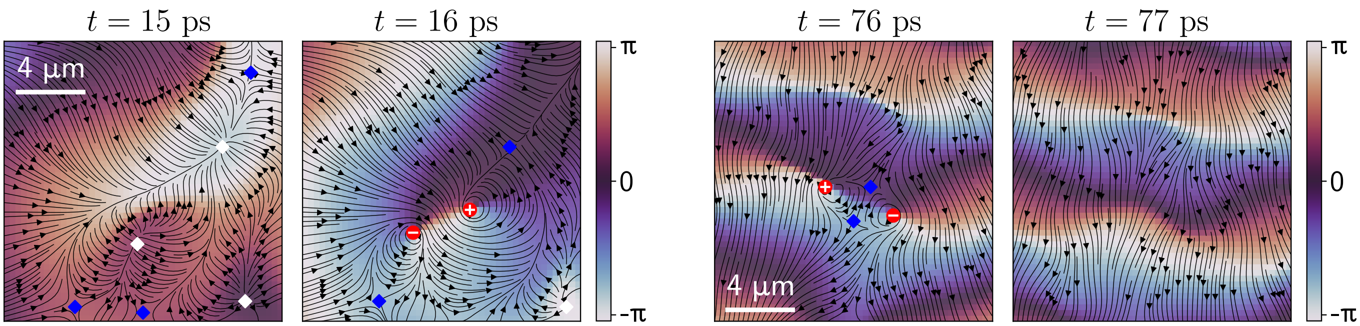


FIG. S2. (left) Experimental snapshots, taken at times $t = 15$ and $t = 16$ ps, showing the formation of a vortex-antivortex pair starting from two nearby nodes, as indicated by Eq. (S1). The streamlines of the velocity field $\vec{v} = (\hbar/m)\vec{\nabla}\Theta$ are plotted as oriented solid lines, on top of the color-coded phase field $\Theta(x, y)$. (right) Experimental snapshots of streamlines and the phase field taken during stage 2 of the experiment, at times $t = 76$ and $t = 77$ ps, showing the annihilation of two saddles and a vortex-antivortex pair via the Bristol mechanism (S2).

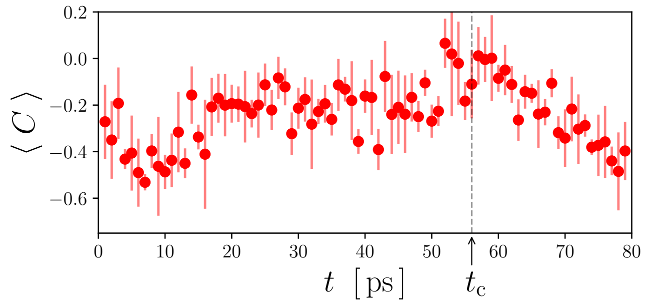


FIG. S3. Experimental correlation function (S3) averaged over 4 realizations plotted as a function of time. The dots correspond to the mean value, the vertical segments are the standard deviations. Adapted from Ref. [3].

observables characterizing the non-linear dynamics in the turbulent superfluid discussed in the main text indicates that $t_c$ is also the time at which the inverse cascade stops and turbulence starts its decay.

A first simple remark is in order: if vortices of the same vorticity are gathered in packs they cannot annihilate since they need to encounter vortices of opposite vorticity to do so. Hence, clustering tends to prevent vortices from annihilating each other. An initial increase followed by a (faster) decrease of clustering is revealed in Fig. S3 which displays the average of the correlation function $C$, defined as [1, 2]

$$C = \frac{1}{V}\sum_{i=1}^{V} c_i, \tag{S3}$$

where $V$ is the total number of vortices and $c_i = 1$ $(-1)$ if the vortex closest to a given vortex $i$ has the same (opposite) vorticity. The largest possible value of the correlation function is $C = +1$ and is reached for perfect clustering. $C = -1$ is associated with the state of lowest energy and (positive) temperature; increasing values of $C$ correspond to higher energetic states of the vortex gas. The figure shows that clustering starts to decrease at the same time $t_c = 56$ ps at which vortex decay sets in. The concomitant decrease of clustering and of the number of vortices is an interesting test of coherence of the point of view we have on the phenomenology of the system, but is not in itself an explanation of the underlying physical mechanism. The results discussed in the main text suggest that it is the incompressible component of the kinetic energy which triggers both phenomena.

## LOW-ENERGY DATA SET

The data presented in the main text correspond to a turbulent regime in which a high-energy polariton superfluid is injected against a potential barrier. We consider in this section a data set obtained at relatively low injection energy: $E = E^{\text{low}} = 0.21$ meV here, instead of $E^{\text{high}} = 1.20$ meV in the main text (both sets of data are extracted form the experiment of Ref. [3]).

The low-energy experimental results for the number of critical points, presented in Fig. S4, display a tendency to saturate: from $t = 60$ ps on, $V(t)$, $S(t)$, and $N(t)$ vary quite slowly. To emulate this behavior, the dimensionless dynamical system for $V$, $S$ and $N$ should have a fixed point. We recall the corresponding equations here for completeness [Eqs. (4) of the main paper]:

$$\frac{\mathrm{d}v}{\mathrm{d}\tau} = n^2 - \alpha v^2, \qquad \frac{\mathrm{d}s}{\mathrm{d}\tau} = 1 - \gamma n s, \qquad \frac{\mathrm{d}n}{\mathrm{d}\tau} = 1 - n^2 - \gamma n s + \alpha v^2, \tag{S4}$$

where $v = V/N_0$, $S = S/N_0$, $n = N/N_0$, $\tau = t/t_0$ and $\alpha$ and $\gamma$ are re-scaled reaction rates.

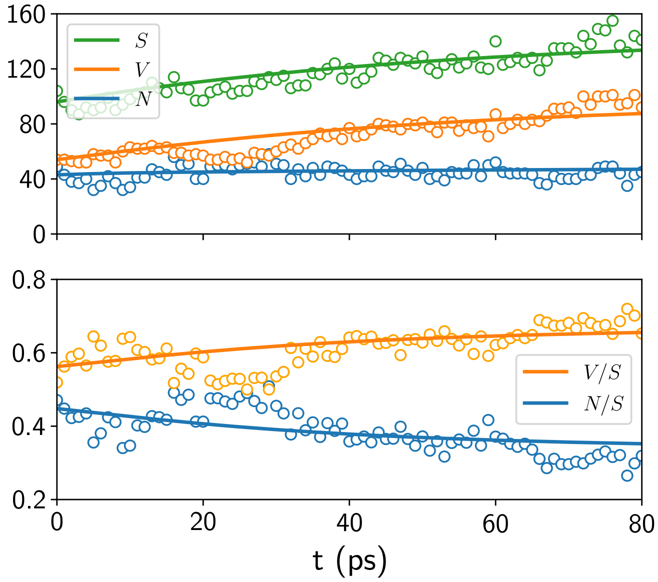


FIG. S4. Comparison of the experimental results of the low-energy data set for the numbers $N(t)$ of nodes, $V(t)$ of vortices, and $S(t)$ of saddles (circles) with the numerical integration of Eqs. (S4) (solid lines).

The parameter $\alpha$ needs to be finite for the system (S4) to have a fixed point. In this case, if we denote as $n_\infty, v_\infty, s_\infty$ the coordinates of the fixed point, defining $\beta = 1/\sqrt{\alpha}$ we get $v_\infty = \beta n_\infty$, $s_\infty = 1/(\gamma n_\infty)$ and

$$n_\infty = \frac{I_{\text{P}0} + \sqrt{I_{\text{P}0}^2 + 4(1+\beta)/\gamma}}{2(1+\beta)}. \tag{S5}$$

In this expression $I_{\text{P}0} = n + v - s$ is the constant value of the rescaled Poincaré index of the whole system ($I_{\text{P}0} = I_{\text{P}}/N_0$). In the limit $I_{\text{P}0}^2 \ll 4(1+\beta)/\gamma$ [4], formula (S5) reads $n_\infty = [\gamma(1+\beta)]^{-1/2}$ and implies that $s_\infty = (1 + \beta)n_\infty$. Comparing the values $v_\infty/n_\infty = \beta$ and $s_\infty/n_\infty =$

$1+\beta$ with the experimental values $V/N \approx 2$ and $S/N \approx 3$ around $t = 60$ ps points to a value $\beta \approx 2$, *i.e.*, $\alpha = 0.25$. We found that the choice $\gamma = 1$, $N_0 = 80$, $t_0 = 27$ ps, and $\alpha = 0.25$ gives a good account of the data set, see Fig. S4.

The system is not here in a turbulent regime such as the one studied in the main text. It is interesting to note that the value $\alpha = 0.25$ corresponds to equality $a = b$ in the node to vortex conversion (S1). Of course we can not ascertain exact equality, but it is clear that $a \simeq b$ which implies that in the non-turbulent setting considered in the present section, the node-to-vortex conversion (S1) is on average in equilibrium. Remarkably, the situation is completely different in the turbulent setting considered in the main text, where $b = 0$ which corresponds to a unidirectional reaction, increasing the number of vortices, as expected in the inverse cascade which occurs during the growth of turbulence.

Also, in the case considered in this section the injection energy $E$ is smaller than in the turbulent case, the number of vortices increases at a lower pace, and the stage of decay (stage 2 in Fig. 3 of the main text) is not reached within the experimental time window. This interpretation of the different behaviors of the two data sets is corroborated by the following evaluation of orders of magnitude: A simple dimensional argument suggests that the characteristic time $t_0$ should scale as $t_0 \propto E^{-1/2}$. And indeed the characteristic times $t_0^{\text{low}}$ and $t_0^{\text{high}}$ for the two sets of data are in a ratio $t_0^{\text{low}}/t_0^{\text{high}} = 27\,\text{ps}/11\,\text{ps} = 2.45$ which is consistent with the value $\sqrt{E^{\text{high}}/E^{\text{low}}} = \sqrt{1.20\,\text{meV}/0.21\,\text{meV}} = 2.39$.


[1] A. C. White, C. F. Barenghi, and N. P. Proukakis, Creation and characterization of vortex clusters in atomic Bose-Einstein condensates, Phys. Rev. A **86**, 013635 (2012).

[2] S. P. Johnstone, A. J. Groszek, P. T. Starkey, C. J. Billington, T. P. Simula, and K. Helmerson, Evolution of large-scale flow from turbulence in a two-dimensional superfluid, Science **364**, 1267 (2019).

[3] R. Panico, P. Comaron, M. Matuszewski, A. S. Lanotte, D. Trypogeorgos, G. Gigli, M. De Giorgi, V. Ardizzone, D. Sanvitto, and D. Ballarini, Onset of vortex clustering and inverse energy cascade in dissipative quantum fluids, Nat. Photonics **17**, 451 (2023).


[4] It can be checked *a posteriori* that this approximation is legitimate: the total experimental Poincaré index is $I_{\text{P}} = \pm 2$ whereas $N_0$ is of order $10^2$: $I_{\text{P}0}^2 \approx 10^{-4}$. The term $4(1+\beta)/\gamma$ is instead of order unity.
